# Supplementary material for: Autonomously revealing hidden local structures in supercooled liquids
Source: arXiv:2003.00586 ancillary file (2020-03-01)
Supplement: Supplementary file 1 [file SI.pdf]

# Supplementary Information
# Autonomously revealing hidden local structures in supercooled liquids

Emanuele Boattini[1], Susana Marín-Aguilar[2], Saheli Mitra[2], Giuseppe Foffi[2], Frank Smallenburg[2], Laura Filion[1]
[1]*Soft Condensed Matter, Debye Institute of Nanomaterials Science, Utrecht Utrecht, Netherlands*
[2]*Université Paris-Saclay, CNRS, Laboratoire de Physique des Solides, 91405 Orsay, France*

## UNSUPERVISED MACHINE LEARNING

In this paper, we employ an unsupervised machine learning (UML) method to classify particles into two groups based on their local environment. As mentioned in the Methods section, we describe the local environment of particle $i$ in terms of a vector $\mathbf{Q}(i)$ of bond order parameters. This vector has length $d = 8$. As clustering particles with similar environments is difficult in such a high-dimensional space, we reduce the dimensionality of this vector using a neural-network-based auto-encoder. A sketch of such an auto-encoder is shown in Fig. S1. Essentially, the auto-encoder is a neural network trained to reproduce its input as its output. The neural network is especially designed to contain a "bottleneck" with a dimensionality lower than the input and output vectors, such that the network is forced to compress the information, and subsequently decompress it again. After training the auto-encoder (which can be done on a single simulation snapshot), we only retain the encoding part of the network, and use it as our dimensionality reducer (as shown in Fig. 1 of the main text). This assigns to each particle a lower-dimensional vector which can be used to group particles with similar environments.

In order to cluster together similar environments in the low-dimensional subspace found by the encoder, we use Gaussian mixture models (GMMs) as implemented in scikit-learn[1]. This allows us to separate the particles into two clusters which differ by their local structure. Based on the resulting classification, we assign to each particle a probability $P_{\text{red}}$ of belonging to a specific one of the two clusters. Note that in principle, the two clusters carry no inherent meaning. However, in order to make our figures consistent, we choose (using hindsight) the red cluster to correspond to the more mobile particles in the system.

In the following, we describe in more detail both the dimensionality reduction and the clustering procedures, which closely follow the method introduced in Ref. [2]. Note that, for all systems analysed in this work, we perform a separate analysis for the two species of particles.

### Nonlinear dimensionality reduction using neural-network-based autoencoders

In order to reduce the dimensionality, i.e. extract the relevant information, of the vectors $\mathbf{Q}(i)$, we use neural-network-based autoencoders[3–7]. An autoencoder is a neural network that is trained to perform the identity mapping, where the network inputs, $\mathbf{Q}(i) \in \mathbb{R}^d$, are approximately reproduced at the output layer, $\hat{\mathbf{Q}}(i) \in \mathbb{R}^d$. The network may be viewed as consisting of two parts: an encoder network, which performs a nonlinear projection of the input data onto a low-dimensional subspace (the bottleneck), $\mathbf{Y}(i) \in \mathbb{R}^c$ with $c < d$, and a decoder network that attempts to reconstruct the input data from the low-dimensional projection. This architecture is represented in Fig. S1.

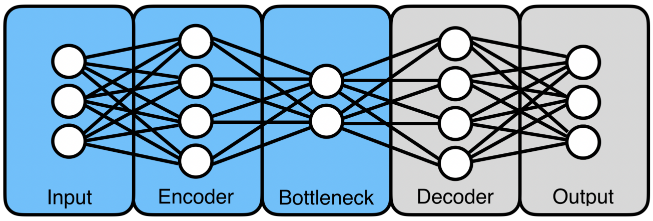


FIG. S1: Architecture of a neural-network based autoencoder. The encoder network (highlighted in blue) finds a low dimensional representation of the input, from which the decoder reconstructs an approximation of the input as output.

By training the autoencoder to perform the input reconstruction task over an ensemble of training examples, the encoder is forced to learn a low-dimensional nonlinear projection that preserves the most relevant features of the data and from which the higher-dimensional inputs can be approximately reconstructed by the decoder.

The number of input and output nodes, $d$, is specified by the dimension of the input vectors. Nonlinearity is achieved by providing both the encoder and the decoder with a fully-connected hidden layer with a nonlinear activation function. In this work, we set the number of nodes in the hidden layers to $5d$ and use a hyperbolic tangent as the activation function. For the bottleneck and output layers, instead, a linear activation function is used.

The internal parameters of the autoencoder, i.e. weights $\mathbf{W} \equiv \{w_j\}$ and biases $\mathbf{B} \equiv \{b_k\}$, which are initialized with the normalized initialization proposed by Xavier in Ref. [8], are optimized during the training by iteratively minimizing the reconstruction error of the input data over a training set of $N$ training examples. Specifically, we consider the mean squared error with the addition of a weight decay regularization term[7] to con-

trol the magnitude of the network weights

$$E(\mathbf{W},\mathbf{B};\{\mathbf{Q}(i)\}) = \frac{1}{N}\sum_{i=1}^{N}\left\|\mathbf{Q}(i)-\hat{\mathbf{Q}}(i)\right\|^2 + \lambda\sum_{j=1}^{M} w_j^2, \tag{S1}$$

where $M$ is the total number of weights, whose value depends on the dimension of the network, and we set $\lambda = 10^{-5}$. The function in Eq. S1 is minimized using mini-batch stochastic gradient descent with momentum[7, 9, 10].

The optimal number of nodes in the bottleneck layer, $c$, which defines the unknown relevant dimensionality of the input data, can be determined by computing the fraction of variance explained (FVE) by the reconstruction,

$$\mathrm{FVE} = 1 - \frac{\sum_{i=1}^{N}\left\|\mathbf{Q}(i)-\hat{\mathbf{Q}}(i)\right\|^2}{\sum_{i=1}^{N}\left\|\mathbf{Q}(i)-\bar{\mathbf{Q}}\right\|^2}, \tag{S2}$$

where $\bar{\mathbf{Q}}$ is the mean input vector, and looking for the existence of an elbow in the FVE as a function of $c$ [11]. To detect the presence of an elbow we use the L-method proposed by Salvador and Chan[12]. Additionally, we require the optimal value of $c$ to be such that the FVE is larger than 75%. With this procedure, we found an optimal dimensionality of $c = 2$ both for the hard sphere and Wahnström systems, while a dimensionality of $c = 4$ was necessary for the Kob-Andersen systems.

Once the autoencoder is trained, the encoder network (highlighted in blue in Fig. S1) alone is retained in order to perform the nonlinear mapping of the input vectors $\mathbf{Q}(i)$ onto the low-dimensional subspace defined by the bottleneck layer, $\mathbf{Y}(i)$.

### Clustering

GMM is a probabilistic model that assumes that the observed data are generated from a mixture of a finite number of Gaussian distributions with unknown parameters. The optimal values of these parameters are found iteratively with the expectation-maximization (EM) algorithm[13] in order to create a probability density function that agrees well with the distribution of the data. In this work, we set the number of Gaussian components in the mixture to two, i.e. we ask the algorithm to group the particles into two clusters based on the largest differences in their local structure. The output of a trained GMM is a list of probabilities, $P_j(i)$, corresponding to the posterior probabilities of the $i$-th observation to arise from the $j$-th component in the mixture model. Here, we arbitrarily label the two clusters as "red" and "white" and refer to these probabilities as $P_{\mathrm{red}}(i)$ and $P_{\mathrm{white}}(i) = 1 - P_{\mathrm{red}}(i)$.

## SANN VS. CUTOFF IN KOB-ANDERSEN

In order to describe the local environment of each particle $i$ in terms of BOPs, needed for $\mathbf{Q}(i)$, we require a definition of what neighbors we include in the bond order calculation. For both hard spheres and Wahnström, we used the definition of nearest neighbour from the solid angle nearest neighbor (SANN) algorithm [14]. This algorithm is known to work well for hard spheres, and as Wahnström is very simliar, we expected it to work well here as well. For Kob-Andersen, we also initially used SANN, but later found that using a tuned fixed cutoff radius worked better. In the following we compare the results of SANN and our cutoff of 1.2 $\sigma_L$. In particular, we analyse a snapshot of a glassy Kob-Andersen mixture at density $\rho^* = 1.2$ and temperature $T^* = 0.5$.

Fig. S2 shows a comparison of the Spearman's rank correlation between the particles' dynamic propensity $D_i$ and their membership probability $P_{\mathrm{fast}}(i)$ obtained by using either SANN or a fixed a cutoff radius.

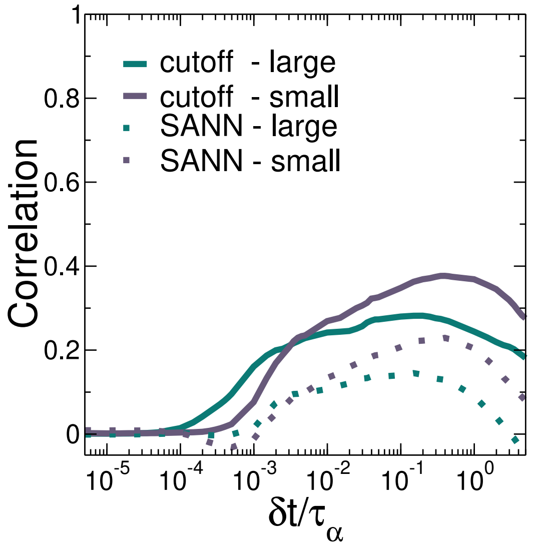


FIG. S2: Comparison of the Spearman's rank correlation between the particles' dynamic propensity $D_i$ and their membership probability $P_{\mathrm{fast}}(i)$ obtained by using either SANN or a cutoff radius of $r_c = 1.2\sigma_L$ for both large and small particles.

## DIMENSIONALITY REDUCTION IN THE WAHNSTRÖM MIXTURE

In order to demonstrate the effect of the dimensionality reduction, we show in Fig. S3a a scatterplot of all local environments of large particles in the Wahnström system at density $\rho^* = 0.81$ and temperature $T^* = 0.7$. For each particle, the encoding part of the auto-encoder has been used to reduce the dimensionality of the vector $\mathbf{Q}$ to two dimensions. As a result, the information

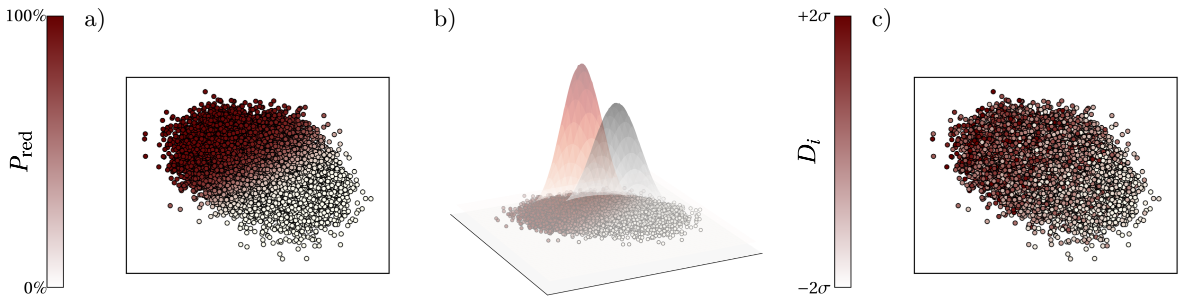


FIG. S3: **a)** Scatterplot of the local descriptors of all large particles in the Wahnström after dimensionality reduction. The points are colored according to their value of $P_{\mathrm{red}}$. **b)** Same scatterplot, with a representation of the two Gaussians found by the clustering. **c)** Same scatterplot, but with points colored according to the dynamic propensity measured at the time with the maximum correlation. Note that the particles are colored according to their deviation from the mean dynamic propensity, in units of the standard deviation $\sigma$. **c)** Same as (a) with a representation of the two Gaussians found by the clustering.

retained by the auto-encoder can be plotted as a point in 2D space for each particle. Using the Gaussian Mixture Model, we classify this set of points into two clusters (white and red), corresponding to two Gaussian distributions of points (Fig. S3b). The connection to dynamics can also be clearly visualized in this reduced space, by coloring particles according to their dynamic propensity (Fig. S3c). This leads to a clear gradient in coloring, indicating that the faster particles (red) lie predominately in the top left cluster, while the slow particles lie in the bottom right one.

## DYNAMIC PROPENSITY CORRELATIONS FOR SMALL PARTICLES

In the main text, we report the correlation between $P_{\mathrm{red}}$ and dynamic propensity for the large particles in all three of our glass forming models at different degrees of supercooling. For completeness, in Fig. S4 we show the same data for the small particles, where we observe approximately the same results.

## CHARACTERIZING THE LOCAL STRUCTURE OF THE DIFFERENT CLUSTERS

An intriguing question is whether we can learn from the UML approach what the nature of the detected structural heterogeneities is. As the UML is based on a description of local environments in terms of bond order parameters [15], a natural question to ask is how the two identified clusters differ in terms of their BOPs. In Fig. S5, we plot the mean value of all bond order parameters $q_1, \cdots, q_8$ for both clusters, in the three systems depicted in Fig. 2 of the main text. Perhaps surprisingly, we do not observe dramatic differences in the average bond order parameters of the two clusters. Small variations are seen in $q_4$, $q_5$, $q_6$, and $q_8$ for hard spheres and Wahnström, while the variations in Kob-Andersen involve the BOPs $q_3$, $q_4$, $q_5$, and $q_8$. In all cases, the fast particles appear to correspond to higher overall bond order.

Another useful tool for examining the local structure of supercooled liquids is the detection of locally favored structures (LFS). In particular, the Topological Cluster Classification (TCC) algorithm [16] has been manually constructed to recognize low-energy (or high-packing) structures in a few model systems. Here, we use the TCC algorithm to count for each particle the number of clusters it is involved in of each type detected by the algorithm. We then calculate the correlation between the number of clusters of a given type a particle is a part of, and $P_{\mathrm{red}}$ as calculated by our UML approach. Note that in its original form, TCC does not accurately count simple clusters (specifically tetrahedra, square pyramids, and pentagonal pyramids) which are subsumed into larger combinations of such clusters. Here we have adapted the algorithm to correct for this choice.

In Fig. S6, we show the correlation between the number of detected clusters for each particle and its value of $P_{\mathrm{red}}$, for all three model systems shown in Fig. 2 of the main text. Clearly, there are strong correlations between membership of TCC clusters and $P$red in both the hard-sphere and Wahnström models. Interestingly, for both of these systems, the fast (red) group correlates strongly with TCC clusters involving square pyramids, highlighted in blue. This includes the pure square pyramid (5B), the BCC unit cell (BCC_9), the double square pyramid (6A), and the 8K, 9K, and 9A clusters, all of which consist largely of connected square pyramidal subclusters. In contrast, the red group correlates *negatively* with a large selection of TCC clusters that consist of connected tetrahedra. This includes e.g. the pure tetrahedron (4A), double tetrahedron (5A), icosahedron (13A), defective icosahedron (10B), and the pentagonal bipyramid (7A, consists of 5 tetrahedra). The only non-tetrahedral TCC cluster that correlates negatively with $P_{\mathrm{red}}$ is the 6B cluster, which consists of a five-ring capped

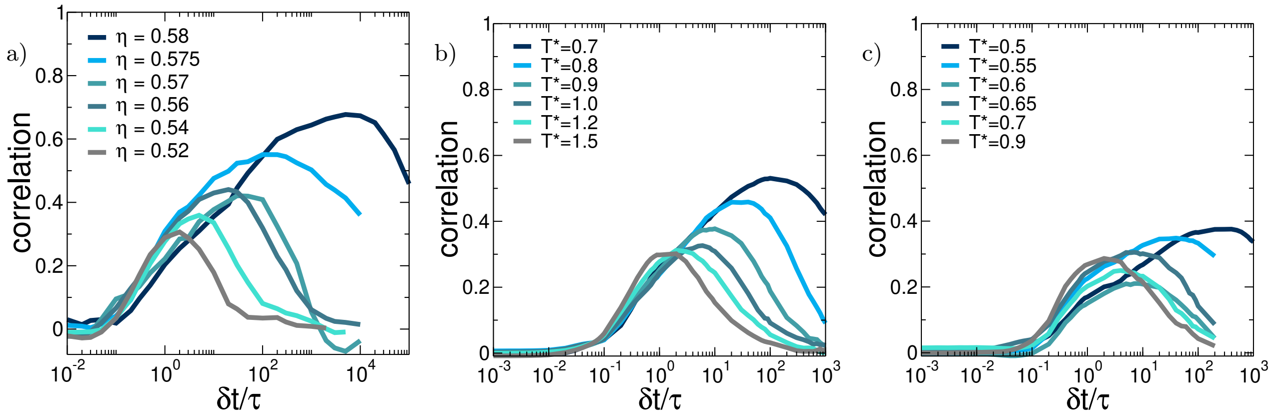


FIG. S4: Correlation between the locally averaged $\bar{P}$red and dynamic propensity for small particles for a) hard spheres, b) Wahnström and c) Kob-Andersen. Note that the averaging radius for $\bar{P}$red is $2\sigma_L$ in all cases.

with a single sphere. This cluster is essentially half a pentagonal bipyramid (7A), and hence is also expected to correlate strongly with tetrahedra.

Hence, our observation is that the UML approach labels highly tetrahedral structures as “red”, and structures containing square pyramids as “white”. Subsequently, these clusters correlate strongly with local dynamics, as demonstrated in the main text. The observation that tetrahedra and their combinations are slow is consistent with the idea that (defective) icosahedra [17–19] and tetrahedra [20, 21] play an important role in slowing down supercooled liquids. Here, the UML results demonstrate that (for the hard-sphere and Wahnström models) the largest structural variation in the system corresponds to a competition between tetrahedra and square pyramids, which can then be linked to slow and fast dynamics, respectively.

For the Kob-Andersen model, the results are less clearcut. Broadly speaking, the strongest negative correlations with $P_{\mathrm{red}}$ are still found for polytetrahedral clusters, but all correlations are relatively weak. Surprisingly, *none* of the clusters found by TCC show significant positive correlation with $P_{\mathrm{red}}$. Clearly, the UML approach is capable of picking up on local structures not found by TCC, and considers these part of the “red” cluster.


[1] Pedregosa, F. *et al.* Scikit-learn: Machine learning in Python. *J. Mach. Learn. Res.* **12**, 2825 (2011).

[2] Boattini, E., Dijkstra, M. & Filion, L. Unsupervised learning for local structure detection in colloidal systems. *J. Chem. Phys.* **151**, 154901 (2019).

[3] Rumelhart, D. E., Hinton, G. E. & Williams, R. J. Parallel distributed processing: Explorations in the microstructure of cognition, Vol. 1. chap. Learning Internal Representations by Error Propagation, 318–362 (MIT Press, Cambridge, MA, USA, 1986).

[4] Kramer, M. A. Nonlinear principal component analysis using autoassociative neural networks. *AIChE J.* **37**, 233–243 (1991).

[5] Scholz, M. & Vigário, R. Nonlinear PCA: a new hierarchical approach. In *ESANN* (2002).

[6] Goodfellow, I., Bengio, Y. & Courville, A. *Deep Learning* (The MIT Press, 2016).

[7] Bishop, C. M. *Neural Networks for Pattern Recognition* (Oxford University Press, Inc., New York, NY, USA, 1995).

[8] Glorot, X. & Bengio, Y. Understanding the difficulty of training deep feedforward neural networks. In *Proceedings of the thirteenth international conference on artificial intelligence and statistics*, 249–256 (2010).

[9] Rumelhart, D. E., Hinton, G. E. & Williams, R. J. Learning representations by back-propagating errors. *Nature* **323**, 533 (1986).

[10] Sutskever, I., Martens, J., Dahl, G. & Hinton, G. On the importance of initialization and momentum in deep learning. In *Proceedings of the 30th International Conference on Machine Learning*, 1139–1147 (JMLR, 2013). URL `http://dl.acm.org/citation.cfm?id=3042817.3043064`.

[11] Chen, W., Tan, A. R. & Ferguson, A. L. Collective variable discovery and enhanced sampling using autoencoders: Innovations in network architecture and error function design. *J. Chem. Phys.* **149**, 072312 (2018).

[12] Salvador, S. & Chan, P. Determining the number of clusters/segments in hierarchical clustering/segmentation algorithms. *16th IEEE International Conference on Tools with Artificial Intelligence* 576–584 (2004).

[13] Dempster, A., Laird, N. & Rubin, D. Maximum likelihood from incomplete data via the EM algorithm. *J. R. Stat. Soc. Series B* **39**, 1 (1977).

[14] Van Meel, J. A., Filion, L., Valeriani, C. & Frenkel, D. A parameter-free, solid-angle based, nearest-neighbor algorithm. *J. Chem. Phys.* **136**, 234107 (2012).

[15] Steinhardt, P. J., Nelson, D. R. & Ronchetti, M. Bond-orientational order in liquids and glasses. *Phys. Rev. B* **28**, 784 (1983).

[16] Malins, A., Williams, S. R., Eggers, J. & Royall, C. P. Identification of structure in condensed matter with the topological cluster classification. *J. Chem. Phys.* **139**, 234506 (2013).

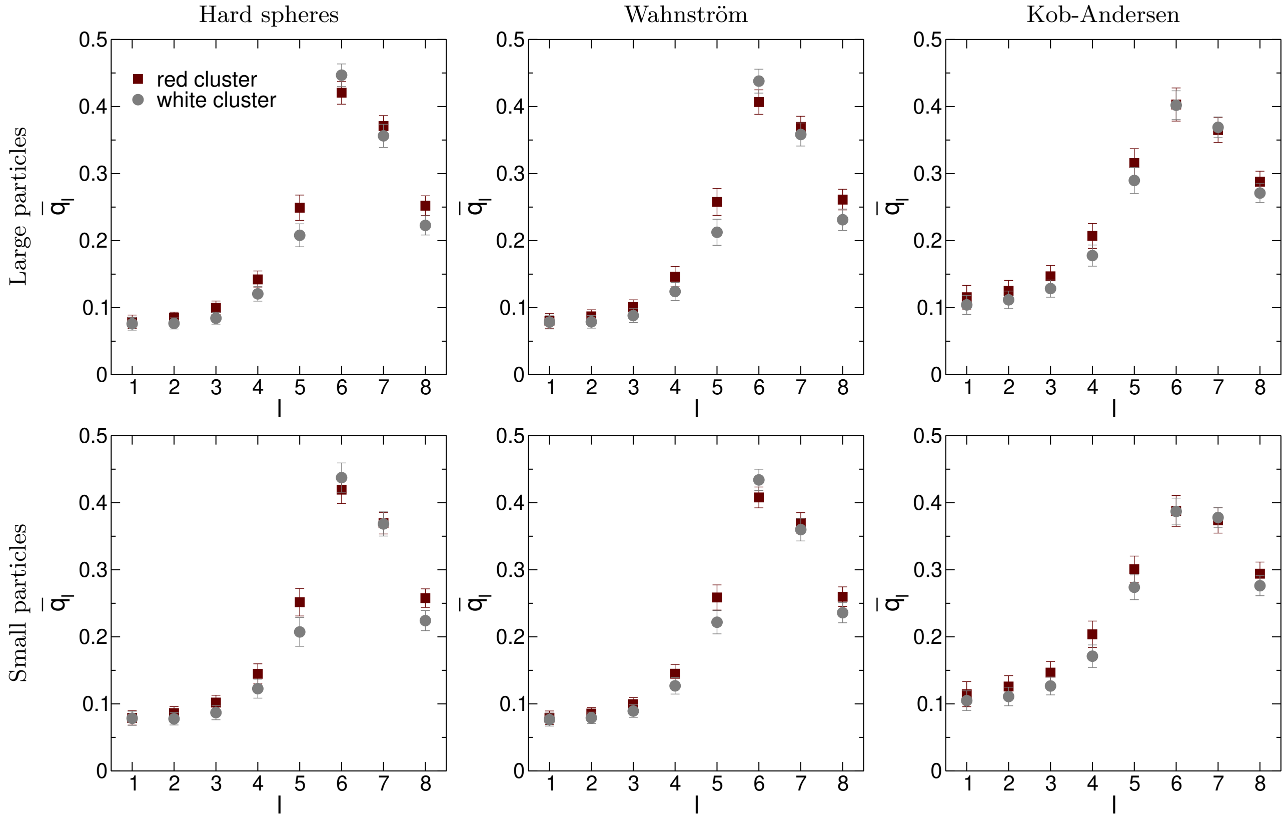


FIG. S5: Mean values of the BOPs for particles in the two clusters identified by the unsupervised learning for all three glass formers. Bars are the standard deviations.

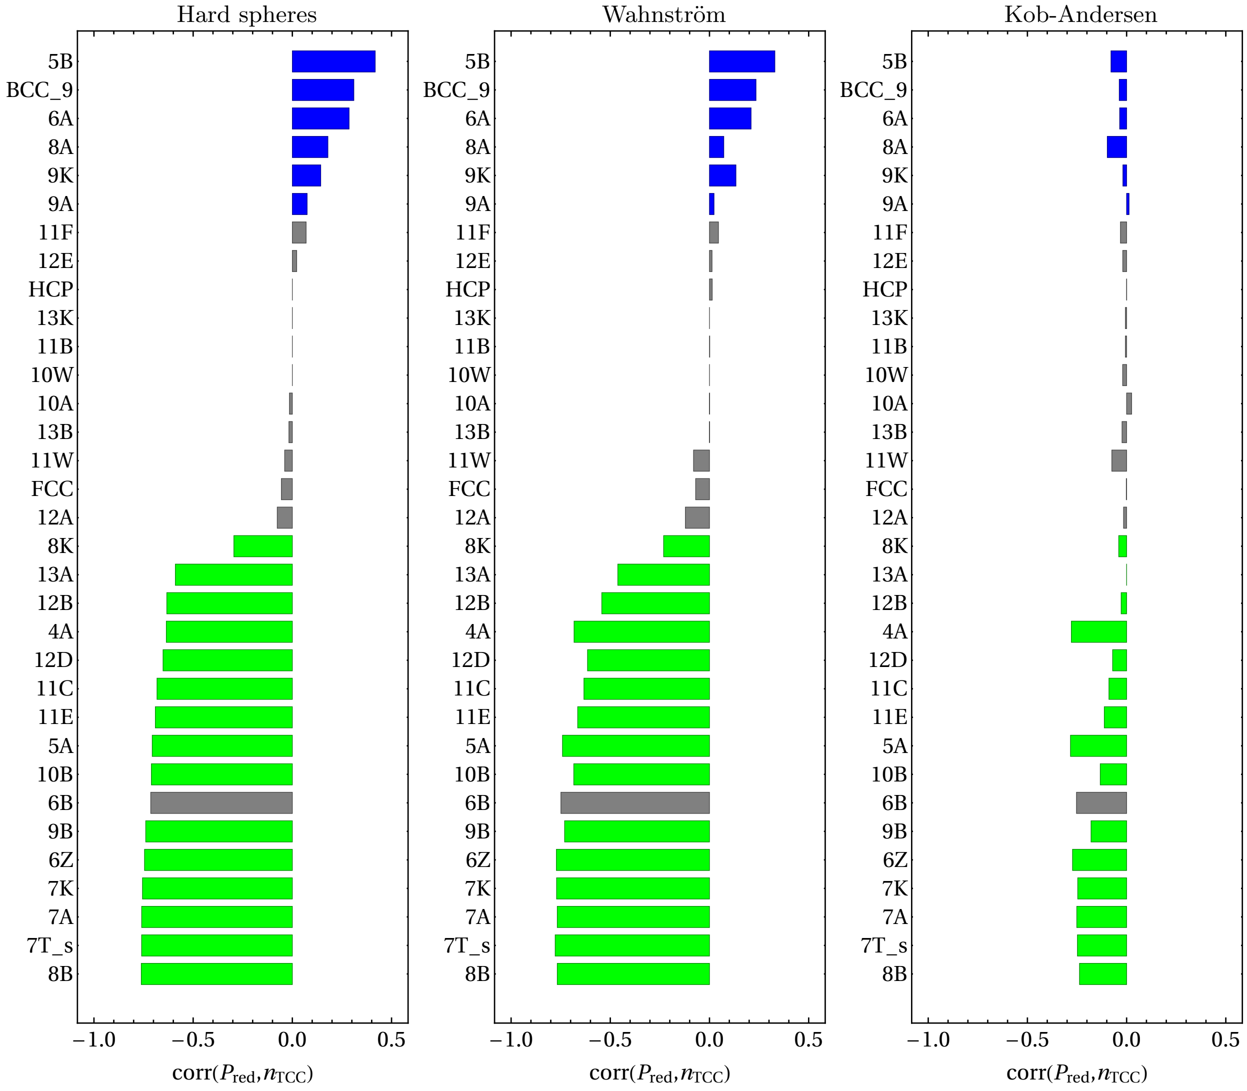


FIG. S6: Correlation between the membership probability $P_{\rm red}$ of a particle and the number of TCC clusters of a given type the particle is involved in, for the three investigated systems. From left to right: hard spheres with packing fraction $\eta = 0.575$, size ratio $q = 0.85$ and composition $x_L = 0.3$, Wahnström at density $\rho^* = 0.81$ and temperature $T^* = 0.7$, and Kob-Andersen at density $\rho^* = 1.2$ and temperature $T^* = 0.5$. The clusters are sorted based on their correlation in the hard sphere model. Green bars indicate clusters that consist of one or more tetrahedral subclusters, while blue bars indicate clusters that consist of one or more square pyramidal subclusters. Gray clusters contain neither (cluster 6B is a single pentagonal pyramid), or both.


[17] Frank, F. C. Supercooling of liquids. *Proc. Royal Soc. A* **215**, 43–46 (1952).

[18] Leocmach, M. & Tanaka, H. Roles of icosahedral and crystal-like order in the hard spheres glass transition. *Nat. Commun.* **3**, 974 (2012).

[19] Royall, C. P. & Williams, S. R. The role of local structure in dynamical arrest. *Phys. Rep.* **560**, 1–75 (2015).

[20] Marín-Aguilar, S., Wensink, H. H., Foffi, G. & Smallenburg, F. Tetrahedrality dictates dynamics in hard spheres. *arXiv:1908.00425* (2019).

[21] Tong, H. & Tanaka, H. Structural order as a genuine control parameter of dynamics in simple glass formers. *Nat. Commun.* **10**, 1–10 (2019).
